# Supplementary material for: Relieving scale disparity in binary black hole simulations
Source: arXiv:2410.22290 ancillary file (2025-09-02)
Supplement: Supplementary file 1 [file supplemental.pdf]

# Convergence Tests and Finite Radius Extraction Errors

In this Supplemental Material, we provide additional details on the convergence analysis and finite radius extraction error assessment associated with the simulations presented in the main letter. These studies verify that the observed waveform behavior is numerically robust, and that the dominant errors originate from the controlled approximations inherent in the worldtube excision method.

## CONVERGENCE ANALYSIS

We have run the eccentric simulation shown in Fig. 2 of the main letter at four different numerical resolutions, denoted `Res 1` through `Res 4` with worldtube radius 0.4 M. The simulation shown in Fig 2 of the main letter is run at the highest resolution, `Res 4`. We then lowered the polynomial expansion order of the solution in each DG element by one order per dimension to obtain an evolution at a lower resolution run which we call `Res 3`. The process was then repeated to get `Res 2` and the lowest resolution, `Res 1`.

The highest resolution `Res 4` is used as a reference solution to compute the absolute angular orbital phase error of the other resolutions at fixed coordinate time. In Fig. 1, we show the evolution of this phase error over the entire inspiral, starting from the point where the self force is fully turned on. The phase naturally accumulates over the course of the simulation as expected. The different resolutions show clear convergence, with higher resolutions showing a lower phase error than lower resolution at almost any time.

We have also included a run at `Res 4` with the smaller worldtube radius of 0.2 M, shown by the red line in the plot. The error of this simulation shows the effect of the worldtube error rather than the numerical resolution. As it is larger than the error of all numerical resolutions, we can conclude that the evolution and phase error estimate presented in the letter really is dominated by the worldtube error which is accurately resolved. We emphasise that the error in these plots is compared at fixed coordinate times as suitable for a convergence test. It is therefore significantly larger than the accumulated phase error quoted in the paper which is calculated at fixed radial phase.

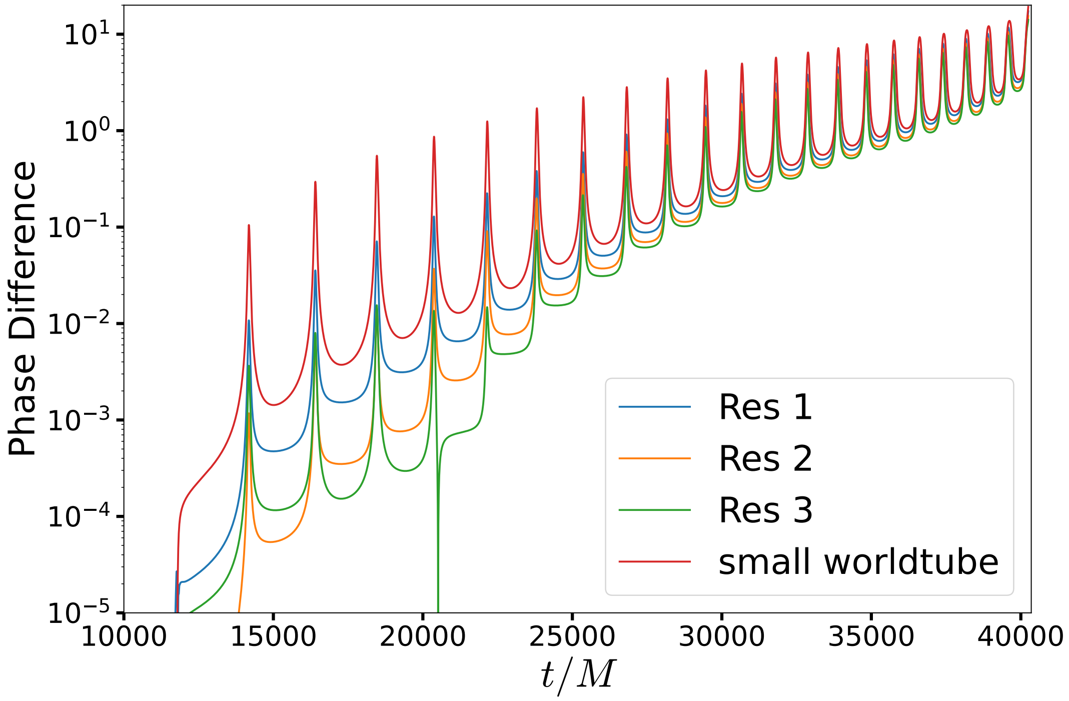


FIG. 1. Absolute phase error relative to the highest resolution (`Res 4`), evaluated at fixed coordinate times. The red curve shows the phase error from a simulation using `Res 4` with a smaller worldtube radius $R = 0.2M$.

Figures 2 and 3 show the same comparison zoomed in to different scales. It shows the same behavior, indicating that we have good convergence at each section of the eccentric orbit.

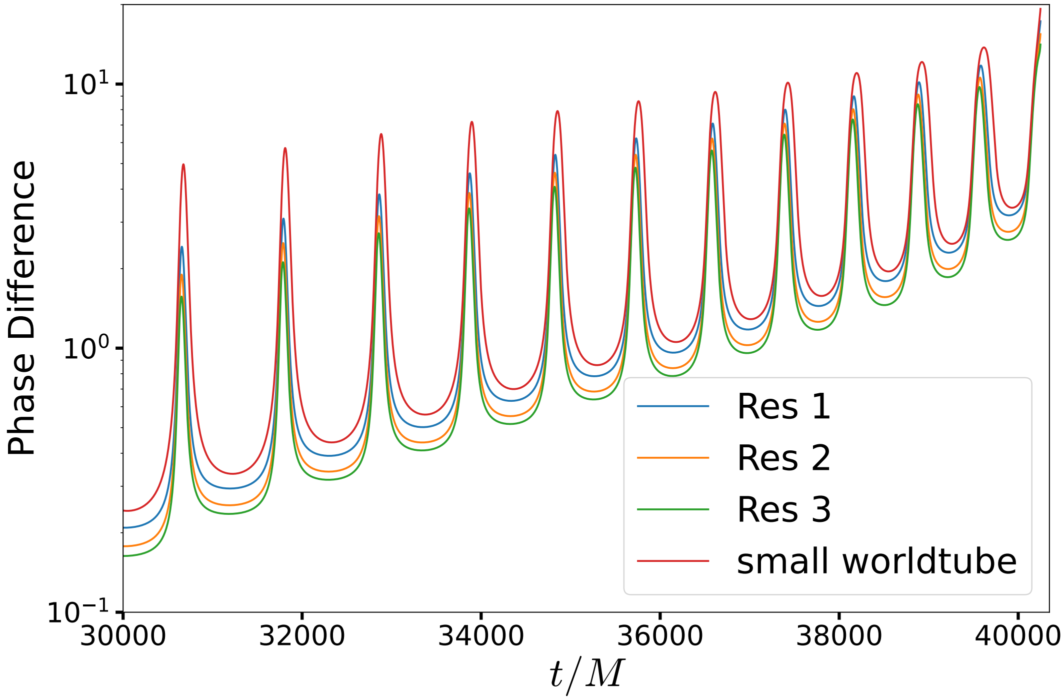


FIG. 2. Zoom-in of Fig. 1 over an early portion of the simulation.

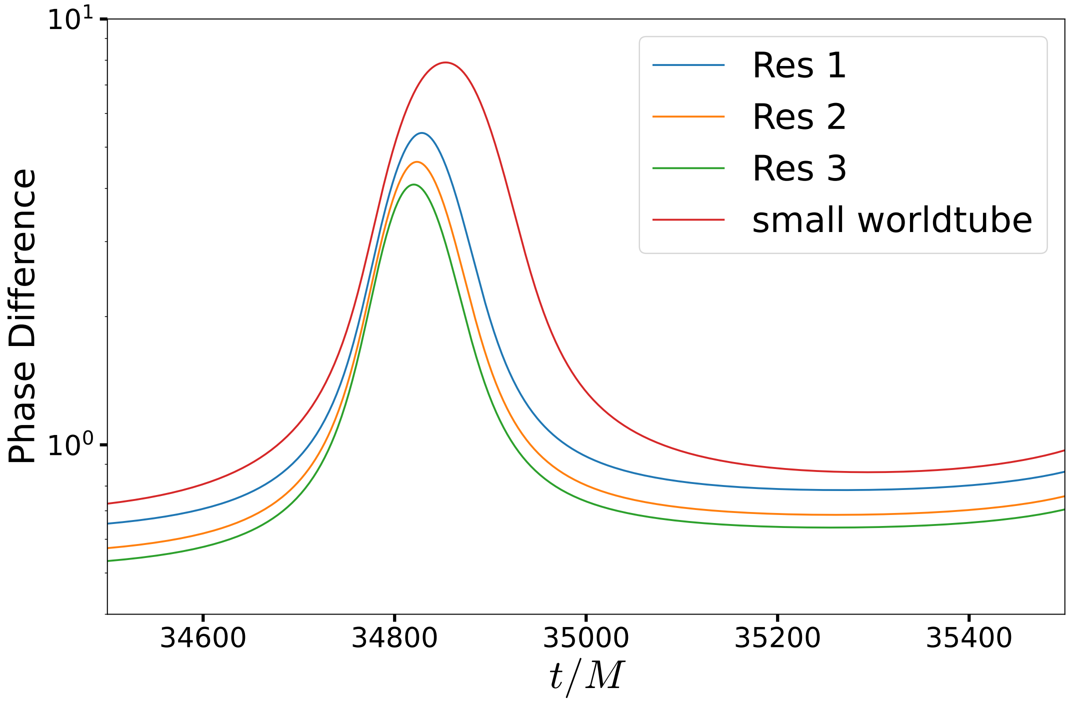


FIG. 3. Zoom-in of Fig. 1 at late times, showing continued convergence.

## FINITE RADIUS EXTRACTION ERROR

We evaluated the error associated with waveform extraction at finite radius by rerunning the eccentric simulation shown in Fig. 2 of the main letter with an enlarged outer boundary located at $R_{\rm out} = 900$ M with additional extraction spheres. Figure 4 compares waveforms extracted at $r = 600$ M and $r = 800$ M.

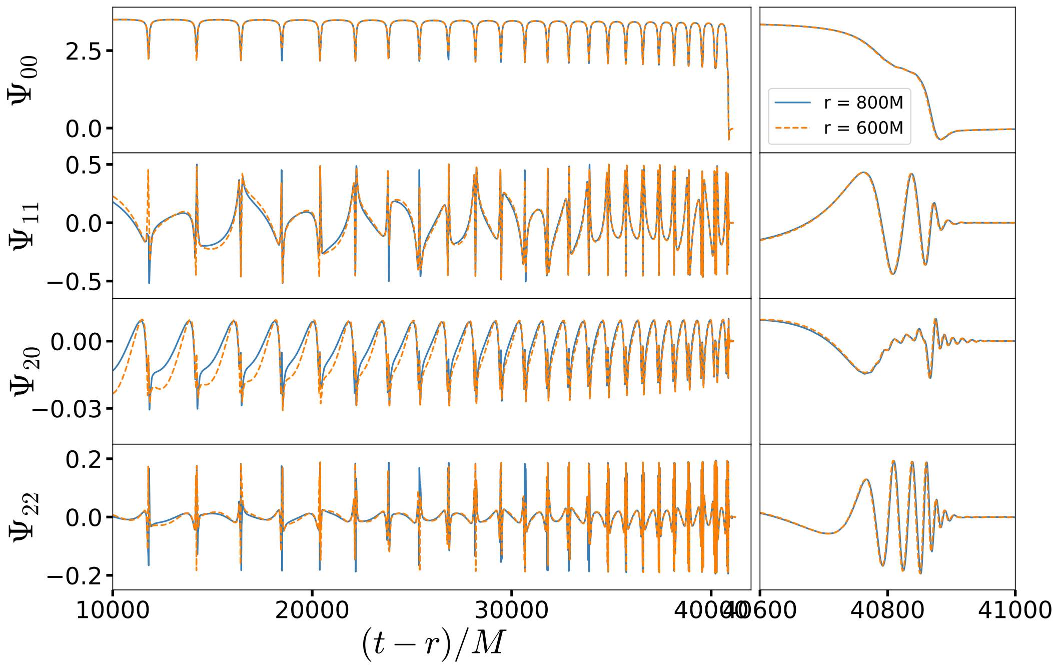


FIG. 4. Comparison of waveforms extracted at $r = 600$ M and $r = 800$ M, showing the expected finite-radius extraction differences.

Small differences between the extracted waveforms are visible, particularly at early times and in the $(2,0)$ mode. These differences are consistent with the expected finite-radius effects. Based on this comparison, we conclude that extraction at $r = 800$ M provides a good approximation to the waveform at future null infinity for the purposes of this letter.
